# Supplementary material for: Phase transition in protocols minimizing work fluctuations
Source: arXiv:1712.05816 ancillary file (2018-04-03)
Supplement: Supplementary file 1 [file SI.pdf]

# Phase transition in protocols minimizing work fluctuations: Supplementary Information

Alexandre P. Solon and Jordan M. Horowitz  
*Physics of Living Systems Group, Department of Physics,  
 Massachusetts Institute of Technology, 400 Technology Square, Cambridge, Massachusetts 02139*  
 (Dated: February 16, 2018)

We derive here the set of Ordinary Differential Equations (ODEs) giving the mean work and work variance obtained for a given (fixed) external protocol and give details on their numerical integration.

## HARMONIC TRAP

In units in which  $k_B T = \gamma = 1$ , the overdamped motion of a Brownian particle in a harmonic trap considered in Eq.(2) (main text) reads  $\dot{x}_t = -k_t x_t + \sqrt{2}\xi_t$ , with  $\xi_t$  a zero-mean Gaussian white noise of unit variance. The spring constant protocol  $k_t$  over the interval  $t \in [0, t]$  evolves from  $k_i$  to  $k_f$ , but we allow for explicit discontinuities at the boundary. Namely,  $k_{0+} \neq k_i$  and  $k_{\tau-} \neq k_f$ , so that there are jumps in the protocol of magnitude  $\Delta_0 k = k_{0+} - k_i$  and  $\Delta_\tau k = k_f - k_{\tau-}$ .

The work obtained in one realization of the protocol can be written as [1]

$$W = \omega_\tau + (\Delta_0 k) \frac{x_0^2}{2} + (\Delta_\tau k) \frac{x_\tau^2}{2}; \quad \omega_\tau = \int_0^\tau \dot{k}_t \frac{x_t^2}{2} dt, \quad (1)$$

explicitly including the work to instantaneously change the spring constant at the initial and final times. Taking the average  $\langle \cdot \rangle$  over noise realizations, the first two moments of the work are expressed as

$$\langle W \rangle = \langle \omega_\tau \rangle + (\Delta_0 k) \frac{\langle x_0^2 \rangle}{2} + (\Delta_\tau k) \frac{\langle x_\tau^2 \rangle}{2}; \quad (2)$$

$$\langle W^2 \rangle = \langle \omega_\tau^2 \rangle + (\Delta_0 k) \langle x_0^2 \omega_\tau \rangle + (\Delta_\tau k) \langle x_\tau^2 \omega_\tau \rangle + \frac{1}{4} [(\Delta_0 k)^2 \langle x_0^4 \rangle + 2(\Delta_0 k)(\Delta_\tau k) \langle x_0^2 x_\tau^2 \rangle + (\Delta_\tau k)^2 \langle x_\tau^4 \rangle]. \quad (3)$$

We can compute each term in Eqs. (2)-(3) as follows: First, we define  $p(x, \omega, t)$  the probability that the particle is found at position  $x$  at time  $t$  having done work  $\omega$  (on the continuous part of the protocol), so that  $\langle \omega_t \rangle = \int dx d\omega \omega p(x, \omega, t)$  and  $\langle \omega_t^2 \rangle = \int dx d\omega \omega^2 p(x, \omega, t)$ . One can show that this distribution evolves as [2]

$$\partial_t p(x, \omega, t) = -\dot{k}_t \frac{x^2}{2} \partial_\omega p + \partial_x (k_t x p + \partial_x p). \quad (4)$$

Using Eq. (4), we can derive a closed set of ODEs satisfied by the terms of Eq. (2)-(3):

$$\begin{aligned} \partial_t \langle \omega_t \rangle &= \frac{\dot{k}_t}{2} \langle x_t^2 \rangle; & \partial_t \langle x_t^2 \rangle &= -2k_t \langle x_t^2 \rangle + 2; \\ \partial_t \langle \omega_t^2 \rangle &= \dot{k}_t \langle x_t^2 \omega_t \rangle; & \partial_t \langle x_t^2 \omega_t \rangle &= 2\langle \omega_t \rangle + \frac{\dot{k}_t}{2} \langle x_t^4 \rangle - 2k_t \langle x_t^2 \omega_t \rangle; \\ \partial_t \langle x_t^4 \rangle &= -4k_t \langle x_t^4 \rangle + 12\langle x_t^2 \rangle; & \partial_t \langle x_0^2 \omega_t \rangle &= \frac{\dot{k}_t}{2} \langle x_t^2 x_0^2 \rangle; \\ \partial_t \langle x_t^2 x_0^2 \rangle &= -2k_t \langle x_t^2 x_0^2 \rangle + 2\langle x_0^2 \rangle. \end{aligned}$$

The particle is assumed to be in equilibrium with the Gaussian distribution  $p(x_0) \propto e^{-k_i x_0^2/2}$  at the beginning of the protocol so that the ODE system is solved with initial condition  $\langle x_0^2 \rangle = 1/k_i$ ,  $\langle x_0^4 \rangle = 3/k_i^2$  and by definition  $\omega_0 = 0$ .

## QUANTUM DOT

The quantum dot evolves due to the exchange of electrons with a particle reservoir at temperature  $T$  and chemical potential  $\mu$ . The rates take the form of Fermi functions and depend on the difference between the dot's energy  $\epsilon_t$  and

the chemical potential  $\mu$ :  $\varepsilon_t = \epsilon_t - \mu$  (in  $k_B T = 1$  units). Thus, the probabilities to be empty  $p_0$  and to be filled  $p_1$  evolve according to the Master equation [3]

$$\partial_t p_0(t) = \frac{1}{1 + e^{-\varepsilon_t}} p_1(t) - \frac{1}{1 + e^{\varepsilon_t}} p_0(t); \quad \partial_t p_1(t) = \frac{1}{1 + e^{\varepsilon_t}} p_0(t) - \frac{1}{1 + e^{-\varepsilon_t}} p_1(t). \quad (5)$$

Probability conservation  $p_0 + p_1 = 1$  allows us to eliminate  $p_0$ , and express the equations of motion totally in terms of  $p \equiv p_1$  as in Eq. (3) of the main text.

As before, we optimize protocols  $\varepsilon_t$  from an initial value  $\varepsilon_i$  to a final value  $\varepsilon_f$ , allowing for discontinuities at the end points of the protocol of magnitude  $\Delta_0 \varepsilon = \varepsilon_{0+} - \varepsilon_i$  and  $\Delta_\tau \varepsilon = \varepsilon_f - \varepsilon_{\tau-}$ . To calculate the work, we write  $s(t)$  for the (fluctuating) state of the quantum dot at time  $t$  such that  $s(t) = 0$  or  $1$  if the dot is respectively empty or occupied. The work done on the system in one realization of the protocol is then

$$W = \omega_\tau + (\Delta_0 \varepsilon) \delta_{s(0)1} + (\Delta_\tau \varepsilon) \delta_{s(\tau)1}; \quad \omega_\tau = \int_0^\tau \dot{\varepsilon}_t \delta_{s(t)1} dt, \quad (6)$$

where  $\delta_{ij}$  is the Kronecker delta function. Averaging over realizations of the process, the first two moments of the work read

$$\langle W \rangle = \langle \omega_\tau \rangle + (\Delta_0 \varepsilon) p_0 + (\Delta_\tau \varepsilon) p_\tau; \quad (7)$$

$$\langle W^2 \rangle = \langle \omega_\tau^2 \rangle + 2(\Delta_0 \varepsilon) \langle \delta_{s(0)1} \omega_\tau \rangle + 2(\Delta_\tau \varepsilon) \langle \delta_{s(\tau)1} \omega_\tau \rangle + (\Delta_0 \varepsilon)^2 p_0 + 2(\Delta_0 \varepsilon)(\Delta_\tau \varepsilon) p(t, 0) + (\Delta_\tau \varepsilon)^2 p_\tau \quad (8)$$

where we used that  $\langle \delta_{s(t)1} \rangle = \langle \delta_{s(t)1}^2 \rangle = p_t$  and introduced the joint probability  $p(t, t') = \langle \delta_{s(t)1} \delta_{s(t')1} \rangle$ .

In the same way as for the harmonic oscillator, we introduce the distribution  $\tilde{p}_0(\omega, t)$  (resp.  $\tilde{p}_1(\omega, t)$ ) as the probability to be in state 0 (resp. 1) at time  $t$ , having done a work  $\omega$  on the system. These are such that  $\langle \omega_t^2 \rangle = \int \omega^2 (\tilde{p}_0 + \tilde{p}_1) d\omega$  and  $\langle \delta_{s(t)1} \omega_t \rangle = \int \omega \tilde{p}_1 d\omega$  and evolve as

$$\partial_t \tilde{p}_0(\omega, t) = \frac{1}{1 + e^{-\varepsilon_t}} \tilde{p}_1 - \frac{1}{1 + e^{\varepsilon_t}} \tilde{p}_0; \quad \partial_t \tilde{p}_1(\omega, t) = -\dot{\varepsilon}_t \partial_\omega \tilde{p}_1 + \frac{1}{1 + e^{\varepsilon_t}} \tilde{p}_0 - \frac{1}{1 + e^{-\varepsilon_t}} \tilde{p}_1. \quad (9)$$

Using Eq. (9), one can then write a closed set of ODEs, which upon integration will give us the mean work and work variance:

$$\begin{aligned} \partial_t \langle \omega_t \rangle &= \dot{\varepsilon}_t p_t; & \partial_t \langle \omega_t^2 \rangle &= 2\varepsilon_t \langle \delta_{s(t)1} \omega_t \rangle; \\ \partial_t \langle \delta_{s(t)1} \omega_t \rangle &= \dot{\varepsilon}_t p_t + \frac{1}{1 + e^{\varepsilon_t}} \langle \omega_t \rangle - \langle \delta_{s(t)1} \omega_t \rangle; & \partial_t \langle \delta_{s(0)1} \omega_t \rangle &= \dot{\varepsilon}_t p(t, 0); \\ \partial_t p(t, 0) &= -p(t, 0) + \frac{1}{1 + e^{\varepsilon_t}}. \end{aligned}$$

These should be supplemented with the equilibrium initial condition  $p_0 = (1 + e^{\varepsilon_i})^{-1}$ ,  $p(0, 0) = 1$  and  $\omega_0 = 0$ .

Because of the symmetry between the empty and filled states of the quantum dot, flipping the protocol  $\varepsilon_t \rightarrow -\varepsilon_t$  changes the average work to  $\langle W \rangle - (\varepsilon_f - \varepsilon_i)$  with the same variance  $\sigma_W^2 = \langle W^2 \rangle - \langle W \rangle^2$ . As a result, the optimal protocols for a lowering of the energy level such that  $\varepsilon_i = \varepsilon$  and  $\varepsilon_f = -\varepsilon$  are simply the opposite of those for an increase of energy  $\varepsilon_i = -\varepsilon$  and  $\varepsilon_f = \varepsilon$ . The structure of the Pareto fronts are thus identical in both cases. An example of this symmetry can be found in [3].

## NUMERICAL PROCEDURE

**Discretization.** We use two levels of discretization. First, the protocol  $\lambda_t$  (either  $k_t$  for the harmonic oscillator or  $\varepsilon_t$  for the quantum dot) is discretized into  $N + 1$  points  $\{\lambda_0, \dots, \lambda_N\}$  with  $\tau = N\Delta t$ .  $\Delta t$  thus sets the precision of the protocol obtained through the optimization. Second, for the numerical integration of the ODEs derived previously, we subdivide each interval  $\Delta t$  in  $n$  smaller steps  $dt = \Delta t/n$ . Over  $\Delta t$ , the protocol is assumed to interpolate linearly as depicted in Fig. 1. The integration is performed using 4th order Runge-Kutta time stepping.

**Gradient descent in protocol space.** Starting from an initial protocol  $\{\lambda_0, \dots, \lambda_N\}$ , the mean work and work variance are computed by integrating the corresponding set of ODEs. A change in one point of the protocol  $\lambda_k \rightarrow \lambda_k + \sigma_\lambda \xi$  is then proposed, with  $\xi$  a Gaussian random number of zero mean and unit variance. The parameter  $\sigma_\lambda$  is adjusted to optimize the efficiency of the gradient descent. The move is then accepted if it decreases the optimization function, as described in the main text.

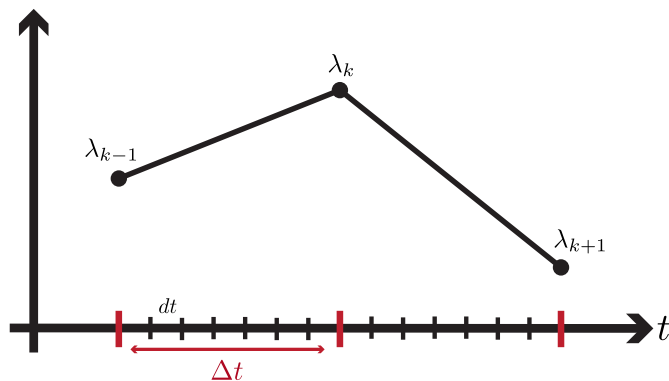

FIG. 1. Illustration of the two levels of discretization with time steps  $\Delta t$  between points in the protocols and a smaller time step  $dt$  for numerical integration.

**Parameters.** We used  $N = 100$  points for all protocols and  $dt = 10^{-3}$ , checking that at the precision required, our results do not depend on these values. When the protocol resulting from the optimization is found to have a sharp interface (such as in Fig. 3 in main text), we rerun the algorithm allowing for an exact discontinuity at this point to avoid numerical errors due to integrating large gradients.

- 
- [1] Ken Sekimoto, *Stochastic energetics*, Vol. 799 (Springer, 2010).
  - [2] A. Imparato, L. Peliti, G. Pesce, G. Rusciano, and A. Sasso, “Work and heat probability distribution of an optically driven brownian particle: Theory and experiments,” *Phys. Rev. E*, **76**, 050101(R) (2007).
  - [3] M. Esposito, R. Kawai, K. Lindenberg, and C. Van den Broeck, “Finite-timethermodynamics for a single-level quantum dot,” *Europhys. Letts.*, **89**, 20003 (2010).
